# Supplementary material for: Using Invalid Instruments on Purpose: Focused Moment Selection and Averaging for GMM
Source: arXiv:1408.0705 source file (2020-11-14)
Supplement: Supplementary file 1 [file c_1equal_OLSvsIV.tex]

\begin{tabular}{r|rrrrrr}
\hline\hline
 &\multicolumn{6}{c}{$\tau$} \\ 
 $\alpha = 0.05$ & $0$ & $1$ & $2$ & $3$ & $4$ & $5$ \\ 
 \hline$0.1$ & $94$ & $94$ & $96$ & $96$ & $94$ & $90$\\ 
$\pi^2\;\;\;$ $0.2$ & $95$ & $95$ & $95$ & $94$ & $91$ & $92$\\ 
$0.3$ & $95$ & $96$ & $94$ & $93$ & $93$ & $94$\\ 
$0.4$ & $96$ & $95$ & $93$ & $93$ & $95$ & $95$\\ 
 \hline 
 \end{tabular}
 
 \vspace{2em} 
 
\begin{tabular}{r|rrrrrr}
\hline\hline
 &\multicolumn{6}{c}{$\tau$} \\ 
 $\alpha = 0.1$ & $0$ & $1$ & $2$ & $3$ & $4$ & $5$ \\ 
 \hline$0.1$ & $90$ & $90$ & $91$ & $89$ & $85$ & $81$\\ 
$\pi^2\;\;\;$ $0.2$ & $91$ & $91$ & $89$ & $85$ & $84$ & $86$\\ 
$0.3$ & $92$ & $91$ & $88$ & $86$ & $87$ & $90$\\ 
$0.4$ & $92$ & $90$ & $87$ & $87$ & $90$ & $91$\\ 
 \hline 
 \end{tabular}
 
 \vspace{2em} 
 
\begin{tabular}{r|rrrrrr}
\hline\hline
 &\multicolumn{6}{c}{$\tau$} \\ 
 $\alpha = 0.2$ & $0$ & $1$ & $2$ & $3$ & $4$ & $5$ \\ 
 \hline$0.1$ & $86$ & $84$ & $77$ & $70$ & $68$ & $68$\\ 
$\pi^2\;\;\;$ $0.2$ & $86$ & $83$ & $75$ & $72$ & $72$ & $77$\\ 
$0.3$ & $86$ & $81$ & $74$ & $73$ & $78$ & $81$\\ 
$0.4$ & $86$ & $79$ & $75$ & $77$ & $81$ & $81$\\ 
 \hline 
 \end{tabular}
