# Supplementary material for: Using Invalid Instruments on Purpose: Focused Moment Selection and Averaging for GMM
Source: arXiv:1408.0705 source file (2020-11-14)
Supplement: Supplementary file 2 [file c_1equal_chooseIVs.tex]

\begin{tabular}{r|rrrrrr}
\hline\hline
 &\multicolumn{6}{c}{$\tau$} \\ 
 $\alpha = 0.05$ & $0$ & $1$ & $2$ & $3$ & $4$ & $5$ \\ 
 \hline$0.1$ & $96$ & $95$ & $94$ & $94$ & $94$ & $95$\\ 
$\gamma^2\;\;\;$ $0.2$ & $96$ & $96$ & $95$ & $93$ & $93$ & $94$\\ 
$0.3$ & $95$ & $96$ & $95$ & $93$ & $93$ & $92$\\ 
$0.4$ & $95$ & $95$ & $96$ & $94$ & $92$ & $91$\\ 
 \hline 
 \end{tabular}
 
 \vspace{2em} 
 
\begin{tabular}{r|rrrrrr}
\hline\hline
 &\multicolumn{6}{c}{$\tau$} \\ 
 $\alpha = 0.1$ & $0$ & $1$ & $2$ & $3$ & $4$ & $5$ \\ 
 \hline$0.1$ & $92$ & $90$ & $88$ & $88$ & $89$ & $91$\\ 
$\gamma^2\;\;\;$ $0.2$ & $92$ & $91$ & $88$ & $86$ & $87$ & $89$\\ 
$0.3$ & $92$ & $91$ & $89$ & $86$ & $86$ & $87$\\ 
$0.4$ & $91$ & $91$ & $90$ & $86$ & $84$ & $85$\\ 
 \hline 
 \end{tabular}
 
 \vspace{2em} 
 
\begin{tabular}{r|rrrrrr}
\hline\hline
 &\multicolumn{6}{c}{$\tau$} \\ 
 $\alpha = 0.2$ & $0$ & $1$ & $2$ & $3$ & $4$ & $5$ \\ 
 \hline$0.1$ & $84$ & $81$ & $76$ & $77$ & $80$ & $81$\\ 
$\gamma^2\;\;\;$ $0.2$ & $86$ & $82$ & $75$ & $74$ & $77$ & $80$\\ 
$0.3$ & $86$ & $82$ & $76$ & $72$ & $73$ & $78$\\ 
$0.4$ & $86$ & $83$ & $77$ & $72$ & $72$ & $75$\\ 
 \hline 
 \end{tabular}
