# Supplementary material for: Using Invalid Instruments on Purpose: Focused Moment Selection and Averaging for GMM
Source: arXiv:1408.0705 source file (2020-11-14)
Supplement: Supplementary file 8 [file w_1equal_chooseIVs.tex]

\begin{tabular}{r|rrrrrr}
\hline\hline
 &\multicolumn{6}{c}{$\tau$} \\ 
 $\alpha = 0.05$ & $0$ & $1$ & $2$ & $3$ & $4$ & $5$ \\ 
 \hline$0.1$ & $ 99$ & $100$ & $104$ & $106$ & $107$ & $104$\\ 
$\gamma^2\;\;\;$ $0.2$ & $ 98$ & $ 99$ & $103$ & $106$ & $108$ & $109$\\ 
$0.3$ & $ 97$ & $ 98$ & $101$ & $105$ & $109$ & $109$\\ 
$0.4$ & $ 97$ & $ 98$ & $100$ & $103$ & $106$ & $109$\\ 
 \hline 
 \end{tabular}
 
 \vspace{2em} 
 
\begin{tabular}{r|rrrrrr}
\hline\hline
 &\multicolumn{6}{c}{$\tau$} \\ 
 $\alpha = 0.1$ & $0$ & $1$ & $2$ & $3$ & $4$ & $5$ \\ 
 \hline$0.1$ & $ 98$ & $100$ & $105$ & $107$ & $106$ & $104$\\ 
$\gamma^2\;\;\;$ $0.2$ & $ 97$ & $ 99$ & $103$ & $107$ & $110$ & $108$\\ 
$0.3$ & $ 96$ & $ 97$ & $101$ & $106$ & $110$ & $110$\\ 
$0.4$ & $ 96$ & $ 97$ & $101$ & $105$ & $108$ & $110$\\ 
 \hline 
 \end{tabular}
 
 \vspace{2em} 
 
\begin{tabular}{r|rrrrrr}
\hline\hline
 &\multicolumn{6}{c}{$\tau$} \\ 
 $\alpha = 0.2$ & $0$ & $1$ & $2$ & $3$ & $4$ & $5$ \\ 
 \hline$0.1$ & $ 98$ & $101$ & $105$ & $107$ & $106$ & $103$\\ 
$\gamma^2\;\;\;$ $0.2$ & $ 98$ & $ 99$ & $104$ & $109$ & $110$ & $108$\\ 
$0.3$ & $ 96$ & $ 96$ & $103$ & $107$ & $110$ & $111$\\ 
$0.4$ & $ 94$ & $ 95$ & $102$ & $106$ & $111$ & $112$\\ 
 \hline 
 \end{tabular}
