# Supplementary material for: Using Invalid Instruments on Purpose: Focused Moment Selection and Averaging for GMM
Source: arXiv:1408.0705 source file (2020-11-14)
Supplement: Supplementary file 9 [file w_2equal_OLSvsIV.tex]

\begin{tabular}{r|rrrrrr}
\hline\hline
 &\multicolumn{6}{c}{$\tau$} \\ 
 $\alpha = 0.05$ & $0$ & $1$ & $2$ & $3$ & $4$ & $5$ \\ 
 \hline$0.1$ & $121$ & $121$ & $123$ & $125$ & $129$ & $131$\\ 
$\pi^2\;\;\;$ $0.2$ & $123$ & $124$ & $127$ & $129$ & $132$ & $134$\\ 
$0.3$ & $124$ & $125$ & $128$ & $130$ & $132$ & $132$\\ 
$0.4$ & $124$ & $125$ & $128$ & $129$ & $129$ & $128$\\ 
 \hline 
 \end{tabular}
 
 \vspace{2em} 
 
\begin{tabular}{r|rrrrrr}
\hline\hline
 &\multicolumn{6}{c}{$\tau$} \\ 
 $\alpha = 0.1$ & $0$ & $1$ & $2$ & $3$ & $4$ & $5$ \\ 
 \hline$0.1$ & $131$ & $130$ & $134$ & $136$ & $140$ & $142$\\ 
$\pi^2\;\;\;$ $0.2$ & $131$ & $132$ & $136$ & $139$ & $141$ & $142$\\ 
$0.3$ & $132$ & $133$ & $136$ & $138$ & $139$ & $139$\\ 
$0.4$ & $133$ & $134$ & $135$ & $136$ & $136$ & $134$\\ 
 \hline 
 \end{tabular}
 
 \vspace{2em} 
 
\begin{tabular}{r|rrrrrr}
\hline\hline
 &\multicolumn{6}{c}{$\tau$} \\ 
 $\alpha = 0.2$ & $0$ & $1$ & $2$ & $3$ & $4$ & $5$ \\ 
 \hline$0.1$ & $148$ & $150$ & $150$ & $153$ & $158$ & $160$\\ 
$\pi^2\;\;\;$ $0.2$ & $148$ & $149$ & $151$ & $155$ & $156$ & $158$\\ 
$0.3$ & $147$ & $149$ & $150$ & $152$ & $153$ & $151$\\ 
$0.4$ & $146$ & $148$ & $149$ & $149$ & $148$ & $144$\\ 
 \hline 
 \end{tabular}
