# Supplementary material for: Using Invalid Instruments on Purpose: Focused Moment Selection and Averaging for GMM
Source: arXiv:1408.0705 source file (2020-11-14)
Supplement: Supplementary file 10 [file w_2equal_chooseIVs.tex]

\begin{tabular}{r|rrrrrr}
\hline\hline
 &\multicolumn{6}{c}{$\tau$} \\ 
 $\alpha = 0.05$ & $0$ & $1$ & $2$ & $3$ & $4$ & $5$ \\ 
 \hline$0.1$ & $124$ & $125$ & $126$ & $126$ & $126$ & $126$\\ 
$\gamma^2\;\;\;$ $0.2$ & $124$ & $125$ & $127$ & $129$ & $130$ & $130$\\ 
$0.3$ & $122$ & $124$ & $127$ & $129$ & $131$ & $132$\\ 
$0.4$ & $123$ & $124$ & $126$ & $129$ & $131$ & $133$\\ 
 \hline 
 \end{tabular}
 
 \vspace{2em} 
 
\begin{tabular}{r|rrrrrr}
\hline\hline
 &\multicolumn{6}{c}{$\tau$} \\ 
 $\alpha = 0.1$ & $0$ & $1$ & $2$ & $3$ & $4$ & $5$ \\ 
 \hline$0.1$ & $132$ & $132$ & $132$ & $133$ & $133$ & $132$\\ 
$\gamma^2\;\;\;$ $0.2$ & $132$ & $133$ & $135$ & $136$ & $138$ & $137$\\ 
$0.3$ & $132$ & $132$ & $135$ & $137$ & $140$ & $140$\\ 
$0.4$ & $132$ & $132$ & $135$ & $137$ & $140$ & $141$\\ 
 \hline 
 \end{tabular}
 
 \vspace{2em} 
 
\begin{tabular}{r|rrrrrr}
\hline\hline
 &\multicolumn{6}{c}{$\tau$} \\ 
 $\alpha = 0.2$ & $0$ & $1$ & $2$ & $3$ & $4$ & $5$ \\ 
 \hline$0.1$ & $145$ & $145$ & $145$ & $145$ & $144$ & $142$\\ 
$\gamma^2\;\;\;$ $0.2$ & $147$ & $148$ & $150$ & $150$ & $151$ & $150$\\ 
$0.3$ & $147$ & $148$ & $151$ & $153$ & $154$ & $154$\\ 
$0.4$ & $148$ & $148$ & $152$ & $154$ & $155$ & $157$\\ 
 \hline 
 \end{tabular}
