# Supplementary material for: Using Invalid Instruments on Purpose: Focused Moment Selection and Averaging for GMM
Source: arXiv:1408.0705 source file (2020-11-14)
Supplement: Supplementary file 11 [file w_2narrowtau_OLSvsIV.tex]

\begin{tabular}{r|rrrrrr}
\hline\hline
 &\multicolumn{6}{c}{$\tau$} \\ 
 $\alpha = 0.05$ & $0$ & $1$ & $2$ & $3$ & $4$ & $5$ \\ 
 \hline$0.1$ & $132$ & $132$ & $134$ & $136$ & $140$ & $143$\\ 
$\pi^2\;\;\;$ $0.2$ & $133$ & $134$ & $138$ & $142$ & $145$ & $147$\\ 
$0.3$ & $135$ & $136$ & $140$ & $143$ & $145$ & $145$\\ 
$0.4$ & $136$ & $137$ & $141$ & $142$ & $143$ & $142$\\ 
 \hline 
 \end{tabular}
 
 \vspace{2em} 
 
\begin{tabular}{r|rrrrrr}
\hline\hline
 &\multicolumn{6}{c}{$\tau$} \\ 
 $\alpha = 0.1$ & $0$ & $1$ & $2$ & $3$ & $4$ & $5$ \\ 
 \hline$0.1$ & $143$ & $144$ & $146$ & $149$ & $152$ & $157$\\ 
$\pi^2\;\;\;$ $0.2$ & $145$ & $146$ & $150$ & $154$ & $157$ & $159$\\ 
$0.3$ & $146$ & $148$ & $152$ & $155$ & $156$ & $157$\\ 
$0.4$ & $147$ & $150$ & $152$ & $154$ & $153$ & $152$\\ 
 \hline 
 \end{tabular}
 
 \vspace{2em} 
 
\begin{tabular}{r|rrrrrr}
\hline\hline
 &\multicolumn{6}{c}{$\tau$} \\ 
 $\alpha = 0.2$ & $0$ & $1$ & $2$ & $3$ & $4$ & $5$ \\ 
 \hline$0.1$ & $165$ & $166$ & $168$ & $173$ & $177$ & $179$\\ 
$\pi^2\;\;\;$ $0.2$ & $168$ & $168$ & $173$ & $177$ & $180$ & $182$\\ 
$0.3$ & $167$ & $169$ & $173$ & $177$ & $178$ & $177$\\ 
$0.4$ & $168$ & $170$ & $174$ & $174$ & $173$ & $169$\\ 
 \hline 
 \end{tabular}
