# Supplementary material for: Using Invalid Instruments on Purpose: Focused Moment Selection and Averaging for GMM
Source: arXiv:1408.0705 source file (2020-11-14)
Supplement: Supplementary file 12 [file w_2narrowtau_chooseIVs.tex]

\begin{tabular}{r|rrrrrr}
\hline\hline
 &\multicolumn{6}{c}{$\tau$} \\ 
 $\alpha = 0.05$ & $0$ & $1$ & $2$ & $3$ & $4$ & $5$ \\ 
 \hline$0.1$ & $136$ & $137$ & $138$ & $139$ & $140$ & $140$\\ 
$\gamma^2\;\;\;$ $0.2$ & $135$ & $137$ & $139$ & $142$ & $143$ & $144$\\ 
$0.3$ & $134$ & $134$ & $138$ & $142$ & $144$ & $145$\\ 
$0.4$ & $133$ & $134$ & $138$ & $141$ & $144$ & $145$\\ 
 \hline 
 \end{tabular}
 
 \vspace{2em} 
 
\begin{tabular}{r|rrrrrr}
\hline\hline
 &\multicolumn{6}{c}{$\tau$} \\ 
 $\alpha = 0.1$ & $0$ & $1$ & $2$ & $3$ & $4$ & $5$ \\ 
 \hline$0.1$ & $148$ & $148$ & $150$ & $150$ & $150$ & $150$\\ 
$\gamma^2\;\;\;$ $0.2$ & $147$ & $147$ & $150$ & $153$ & $155$ & $155$\\ 
$0.3$ & $145$ & $147$ & $150$ & $153$ & $156$ & $158$\\ 
$0.4$ & $145$ & $146$ & $150$ & $153$ & $156$ & $158$\\ 
 \hline 
 \end{tabular}
 
 \vspace{2em} 
 
\begin{tabular}{r|rrrrrr}
\hline\hline
 &\multicolumn{6}{c}{$\tau$} \\ 
 $\alpha = 0.2$ & $0$ & $1$ & $2$ & $3$ & $4$ & $5$ \\ 
 \hline$0.1$ & $168$ & $168$ & $169$ & $170$ & $170$ & $168$\\ 
$\gamma^2\;\;\;$ $0.2$ & $167$ & $169$ & $171$ & $174$ & $176$ & $175$\\ 
$0.3$ & $167$ & $168$ & $171$ & $176$ & $178$ & $179$\\ 
$0.4$ & $167$ & $167$ & $170$ & $175$ & $178$ & $181$\\ 
 \hline 
 \end{tabular}
